# Supplementary material for: Monolayer polar metals with large piezoelectricity derived from MoSi$_2$N$_4$
Source: arXiv:2304.04209 source file (2023-06-12)
Supplement: Supplementary file 1 [file SupportingInformation.pdf]

# Monolayer polar metals with large piezoelectricity derived from $MoSi_2N_4$

Yan Yin,[†] Qihua Gong,[*,†,‡] Min Yi,[*,†] and Wanlin Guo[†]

†*State Key Laboratory of Mechanics and Control for Aerospace Structures & Key Laboratory for Intelligent Nano Materials and Devices of Ministry of Education & Institute for Frontier Science & College of Aerospace Engineering, Nanjing University of Aeronautics and Astronautics (NUAA), Nanjing 210016, China*

‡*MIIT Key Laboratory of Aerospace Information Materials and Physics & College of Physics, Nanjing University of Aeronautics and Astronautics (NUAA), Nanjing 211106, China*

E-mail: gongqihua@nuaa.edu.cn; yimin@nuaa.edu.cn

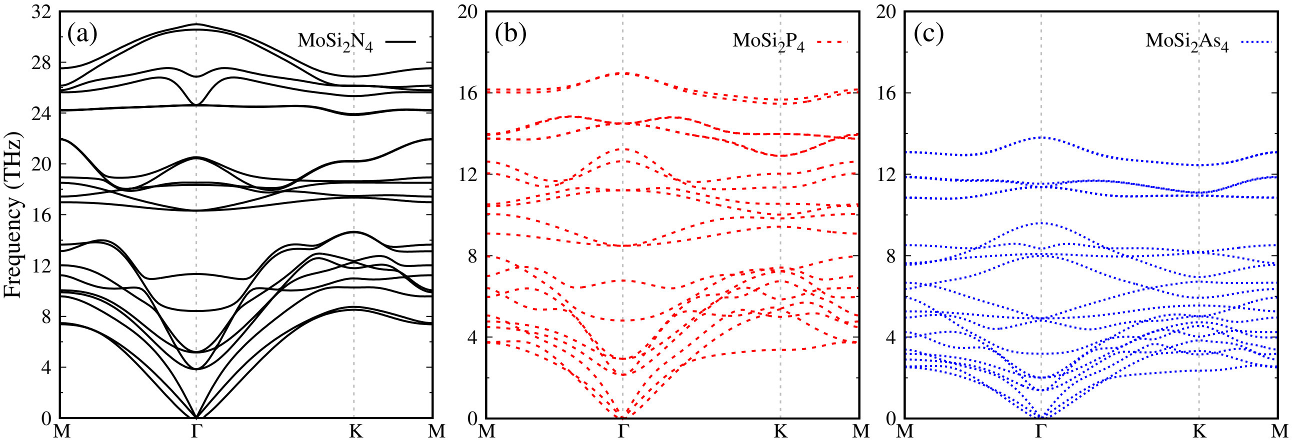


Fig. S1. Phonon dispersion spectra of (a) $MoSi_2N_4$, (b) $MoSi_2P_4$ and (c) $MoSi_2As_4$.

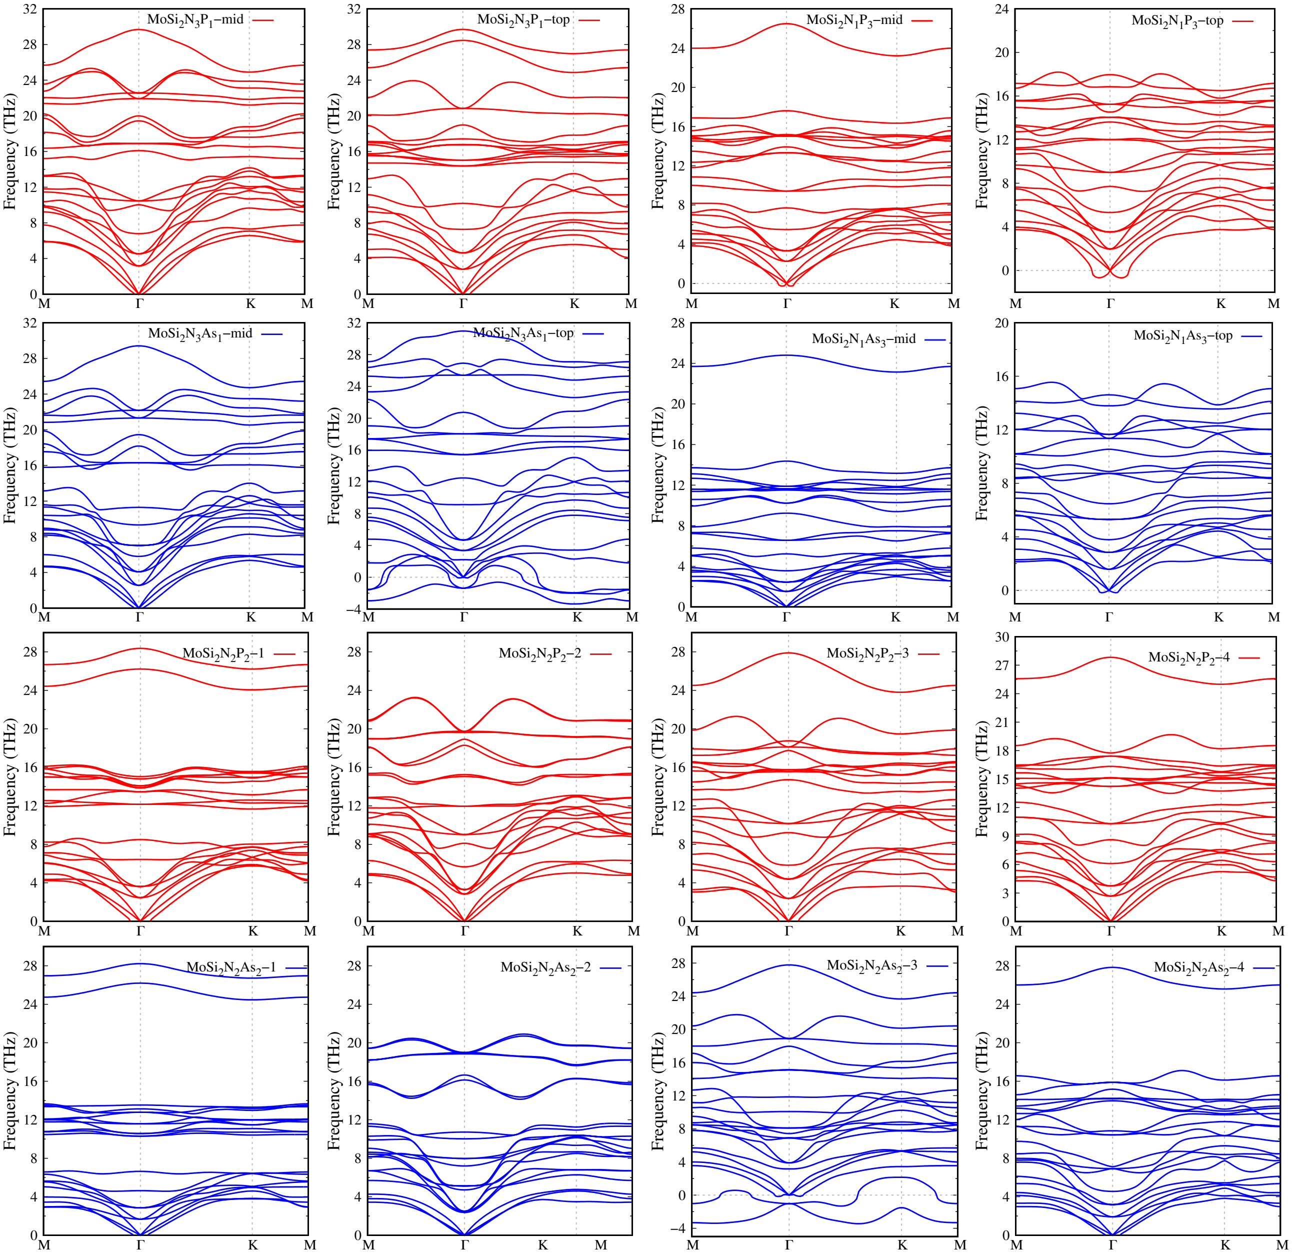


Fig. S2. Phonon dispersion spectra of $MoSi_2N_xZ_{4-x}$ monolayers.

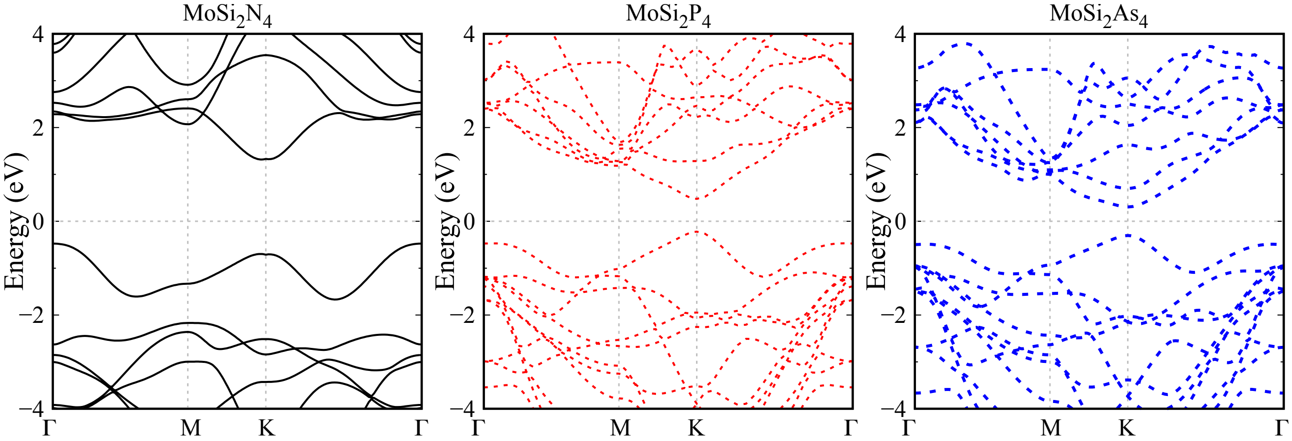

Fig. S3. Band structures of $MoSi_2X_4$ (X=N/P/As).

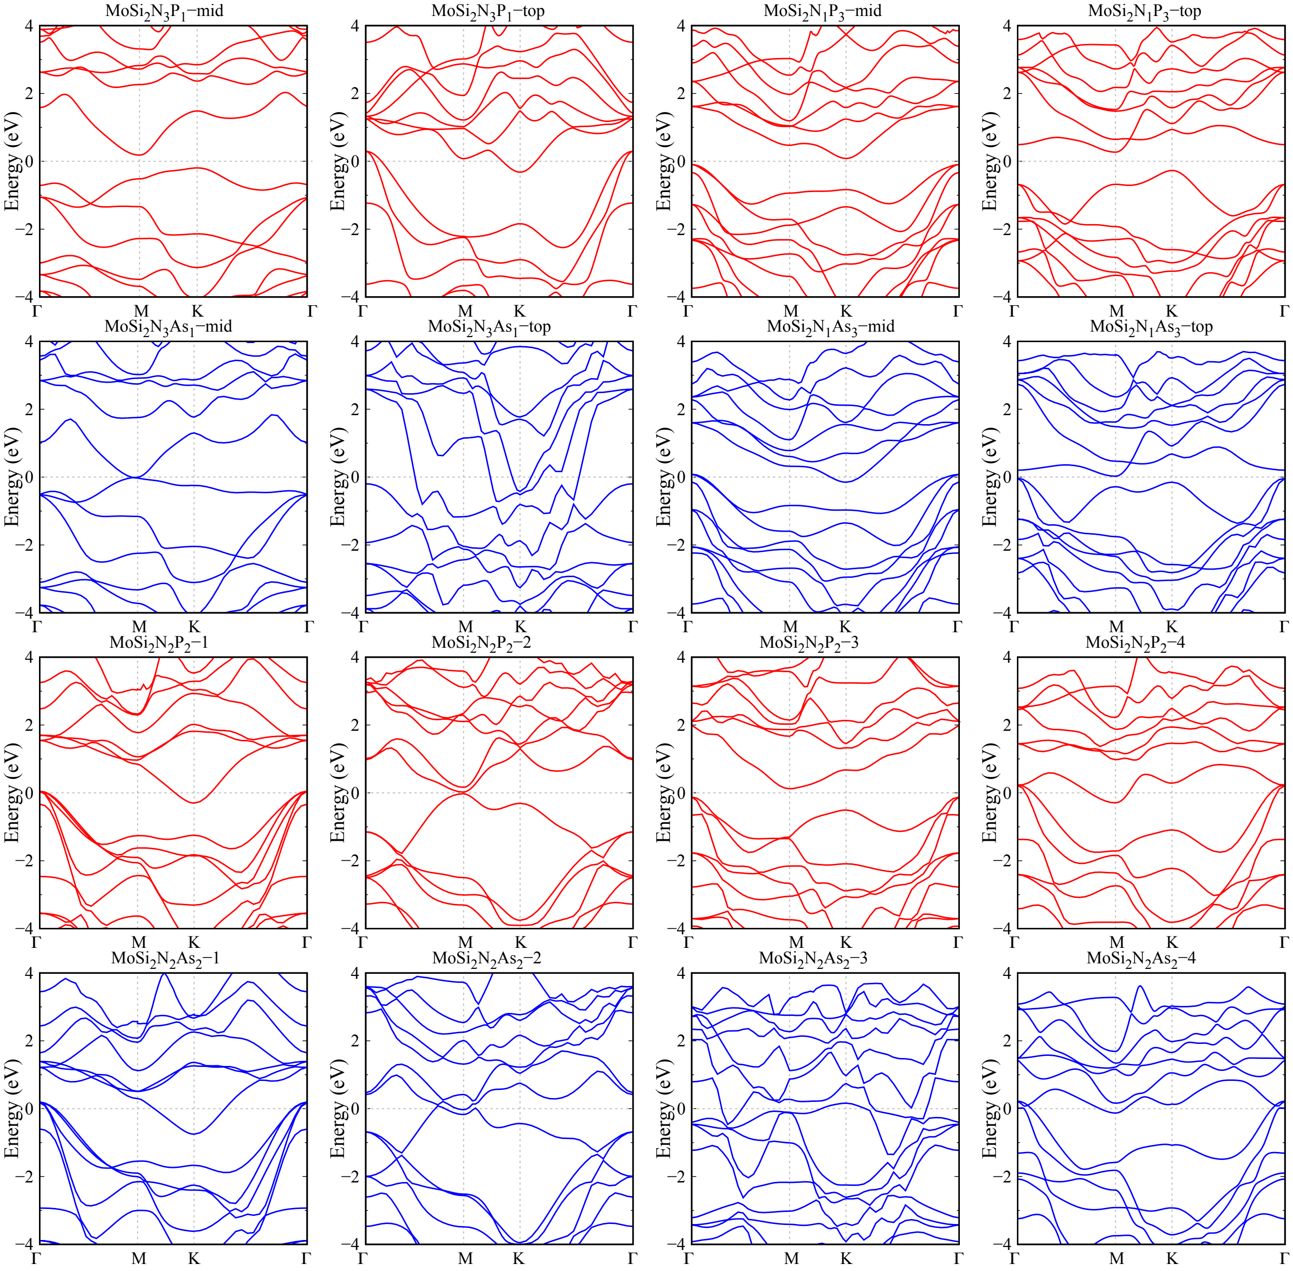


Fig. S4. Band structures of $MoSi_2N_xZ_{4-x}$ monolayers.

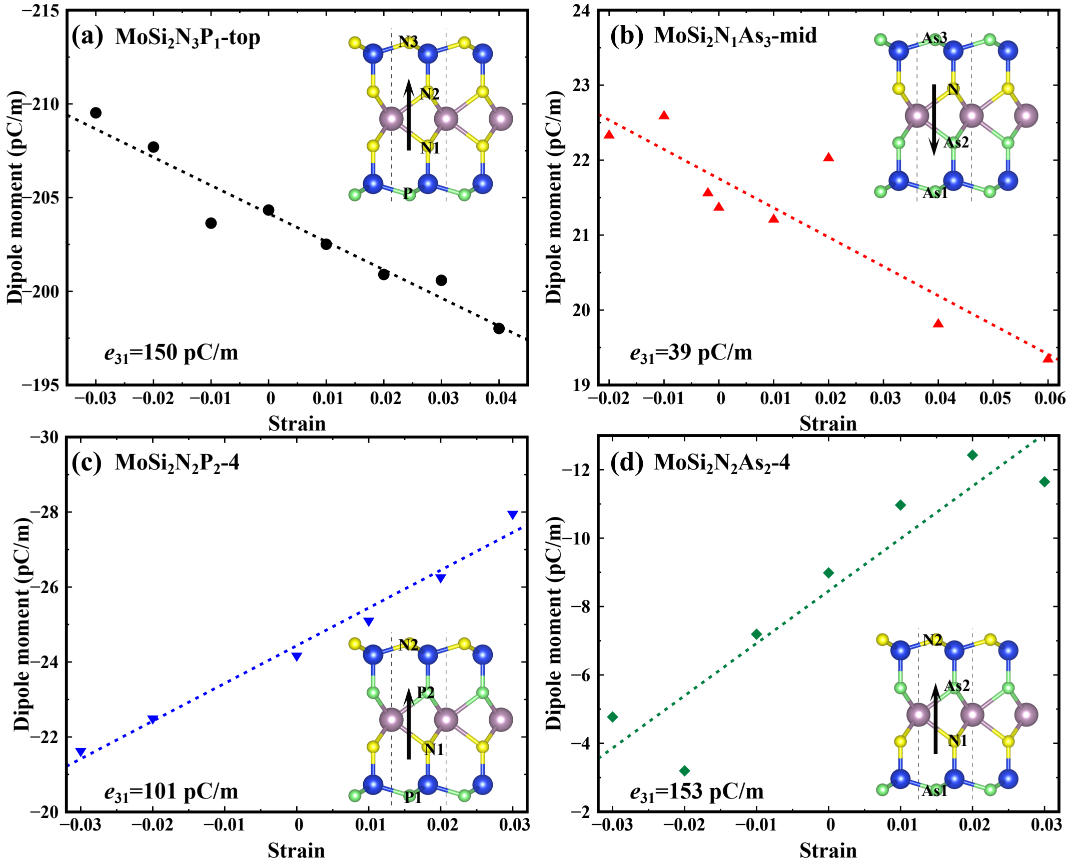


Fig. S5. OOP dipole moment as a function of zigzag uniaxial strain: (a) $MoSi_2N_3P_1$-top, (b) $MoSi_2N_1As_3$-mid, (c) $MoSi_2N_2P_2$-4, (d) $MoSi_2N_2As_2$-4. The inset arrows indicate the dipole moment direction.

Table S1. Structrual parameters of $MoSi_2N_xZ_{4-x}$ monolayers, i.e., lattice constants, thickness ($h$), bond length, formation energy ($E_f$), dynamical stability and band gap from PBE ($E_g^{PBE}$) and HSE ($E_g^{HSE}$)

| Structure | $a=b$ | $h$ | $d_{Z4-Si2}$ | $d_{Z3-Si2}$ | $d_{Z3-Mo}$ | $d_{Z2-Mo}$ | $d_{Z2-Si1}$ | $d_{Z1-Si1}$ | $E_F$ | Dynamics | $E_g^{PBE}$ | $E_g^{HSE}$ |
|---|---|---|---|---|---|---|---|---|---|---|---|---|
| | (Å) | (Å) | (Å) | (Å) | (Å) | (Å) | (Å) | (Å) | (eV/atom) | (Y/N) | (eV) | (eV) |
| $MoSi_2N_4$ | 2.91 | 10.01 | 1.76 | 1.75 | 2.10 | 2.10 | 1.75 | 1.76 | -0.94 | Y | 1.79 | * |
| $MoSi_2P_4$ | 3.47 | 13.17 | 2.25 | 2.24 | 2.46 | 2.46 | 2.24 | 2.25 | -0.34 | Y | 0.70 | * |
| $MoSi_2As_4$ | 3.62 | 13.94 | 2.37 | 2.36 | 2.56 | 2.56 | 2.36 | 2.37 | -0.09 | Y | 0.56 | * |
| $MoSi_2N_3P_1$-mid | 2.98 | 10.92 | 1.79 | 2.23 | 2.37 | 2.12 | 1.75 | 1.79 | -0.28 | Y | 0.38 | 0.96 |
| $MoSi_2N_3P_1$-top | 3.05 | 10.95 | 2.15 | 1.73 | 2.14 | 2.13 | 1.75 | 1.82 | -0.49 | Y | * | * |
| $MoSi_2N_2P_2$-1 | 3.23 | 11.71 | 2.18 | 1.75 | 2.21 | 2.21 | 1.75 | 2.18 | -0.24 | Y | * | * |
| $MoSi_2N_2P_2$-2 | 3.05 | 11.72 | 1.83 | 2.23 | 2.38 | 2.38 | 2.23 | 1.83 | -0.53 | Y | 0.05 | 0.63 |
| $MoSi_2N_2P_2$-3 | 3.14 | 11.66 | 1.87 | 1.76 | 2.16 | 2.39 | 2.23 | 2.16 | -0.39 | Y | 0.24 | 0.88 |
| $MoSi_2N_2P_2$-4 | 3.15 | 11.67 | 1.86 | 2.25 | 2.39 | 2.17 | 1.73 | 2.17 | -0.37 | Y | * | * |
| $MoSi_2N_1P_3$-mid | 3.33 | 12.34 | 2.20 | 1.75 | 2.23 | 2.42 | 2.24 | 2.21 | -0.27 | Y | 0.18 | 0.40 |
| $MoSi_2N_1P_3$-top | 3.26 | 12.33 | 1.93 | 2.24 | 2.42 | 2.42 | 2.23 | 2.19 | -1.35 | N | 0.54 | 0.58 |
| $MoSi_2N_3As_1$-mid | 2.99 | 11.15 | 1.80 | 2.35 | 2.47 | 2.12 | 1.75 | 1.79 | -0.56 | Y | 0.01 | 0.48 |
| $MoSi_2N_3As_1$-top | 2.88 | 12.63 | 1.74 | 1.74 | 2.09 | 2.09 | 1.78 | 3.13 | -0.46 | N | * | * |
| $MoSi_2N_2As_2$-1 | 3.31 | 12.05 | 2.30 | 1.73 | 2.23 | 2.23 | 1.733 | 2.30 | -0.04 | Y | * | * |
| $MoSi_2N_2As_2$-2 | 3.08 | 12.21 | 1.83 | 2.36 | 2.48 | 2.48 | 2.36 | 1.83 | -0.28 | Y | * | * |
| $MoSi_2N_2As_2$-3 | 3.11 | 12.42 | 1.85 | 1.75 | 2.14 | 2.49 | 2.37 | 2.38 | 0.21 | N | * | * |
| $MoSi_2N_2As_2$-4 | 3.20 | 12.04 | 1.89 | 2.38 | 2.49 | 2.18 | 1.71 | 2.29 | -0.14 | Y | * | * |
| $MoSi_2N_1As_3$-mid | 3.49 | 12.77 | 2.34 | 1.74 | 2.27 | 2.54 | 2.36 | 2.33 | -0.05 | Y | * | * |
| $MoSi_2N_1As_3$-top | 3.35 | 12.88 | 1.97 | 2.37 | 2.49 | 2.51 | 2.34 | 2.30 | -0.03 | Y | 0.04 | 0.52 |
